# Supplementary material for: Rb-induced (3x1) and (6x1) reconstructions on Si(111)-(7x7): A LEED and STM study
Source: arXiv:2201.00735 source file (2022-01-03)
Supplement: Supplementary file 1 [file Supplementary.pdf]

# Supplementary Material for:
# Rb-induced reconstructions on Si(111)-(7 × 7): A LEED and STM study

Letizia Ferbel,[1,*] Stefano Veronesi,[1] and Stefan Heun[1]

[1] *NEST, Istituto Nanoscienze-CNR and Scuola Normale Superiore, Piazza San Silvestro 12, 56127 Pisa, Italy*

## Rb DEPOSITION AT ROOM TEMPERATURE (RT) ON THE Si(111)-(7 × 7) SURFACE

### A. LEED

Figure S1 shows a set of LEED patterns, namely of the pristine Si(111)-(7 × 7) sample, after Rb deposition at RT 15 minutes, and after an annealing step at 300°C.

The (7 × 7) pattern is still clearly visible after deposition (see Fig. S1(b)), however, the brightness of the (7 × 7) spots decreases, compared to the pristine silicon sample (Fig. S1(a)). The intensity of the (1 × 1) spots, relative to the silicon bulk, strongly decreases, as well.

After the annealing step (Fig. S1(c)), the intensity of both (7 × 7) and (1 × 1) spots increases, however all the spots result less bright compared to the pristine sample.

In both cases, no additional spots other than the (7×7) spots of the pristine surface are visible, but just a redistribution of their intensities. These observations suggest the presence of a disordered alkali overlayer which does not destroy the periodicity of the underlying (7 × 7) reconstructed Si surface. The LEED pattern obtained after the annealing suggests either an increased order of the surface or partial desorption of the AM.

### B. Preferential adsorption on the (7 × 7) unit cell

In Fig. S2(a) and (c) we show two STM images of the Rb/Si surface obtained after room temperature Rb deposition on the (7×7) silicon surface. The typical triangular pattern observed in the filled state images of the Si(111)-(7×7) surface is still clearly visible and well resolved after Rb deposition. Room temperature deposition of Rb did not induce any new surface reconstruction nor modification of the surface periodicity. Despite the low mobility of Rb atoms at this temperature, we see single atoms or small clusters of Rb atoms preferentially adsorbed on the more reactive faulted half of the (7 × 7) unit cell.

After an annealing step at 300°C (Fig. S2(b) and (d)), the character of the Rb adsorption on the (7 × 7) areas did not change: we still observe preferential adsorption on the faulted half of the (7 × 7) unit cell. In addition, we observe an increase in Rb atoms density near the lower step edge of the terraces (see Fig. S2(b)). Since this was not observed before the annealing, this is a clear indication of an increase in the mobility of the Rb atoms

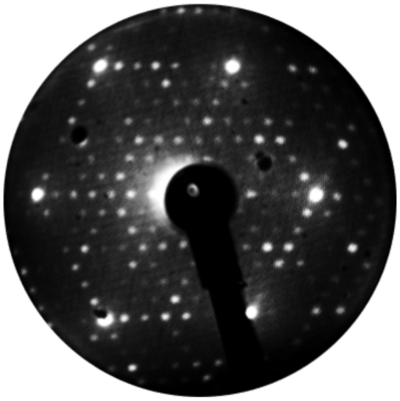

(a) Si(111)-(7 × 7)

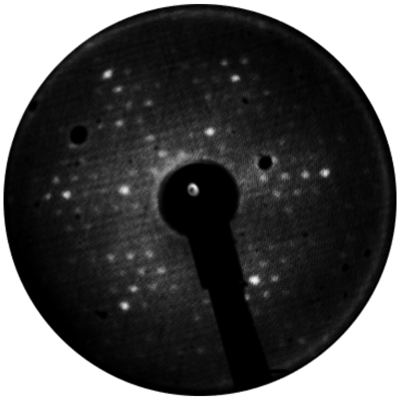

(b) 15 min Rb deposition

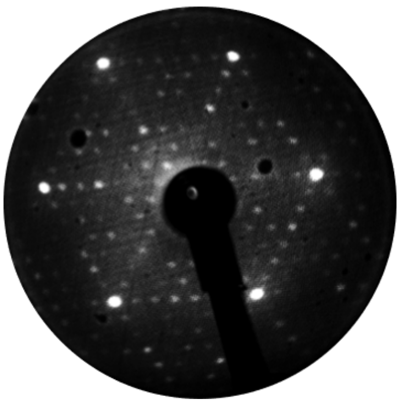

(c) Annealing 300°C

FIG. S1. LEED pattern of (a) Si(111)-(7 × 7), (b) after 15 min room temperature Rb deposition, and (c) after annealing at 300°C. Beam energy: 47 eV.

* letizia.ferbel@sns.it, +39 3466079369

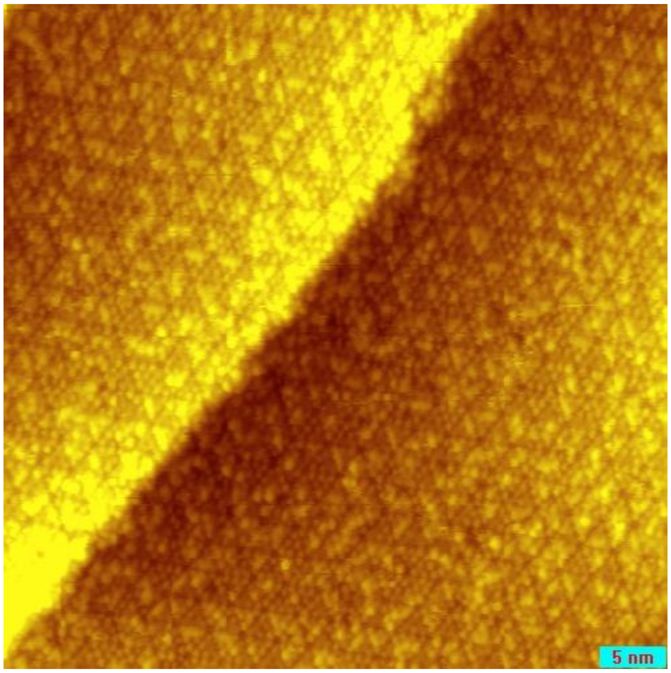


(a) RT deposition

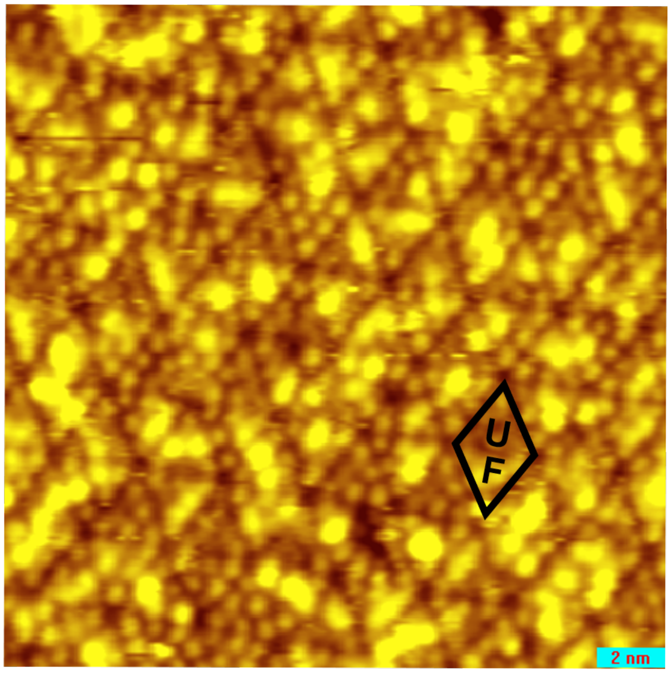


(b) RT deposition

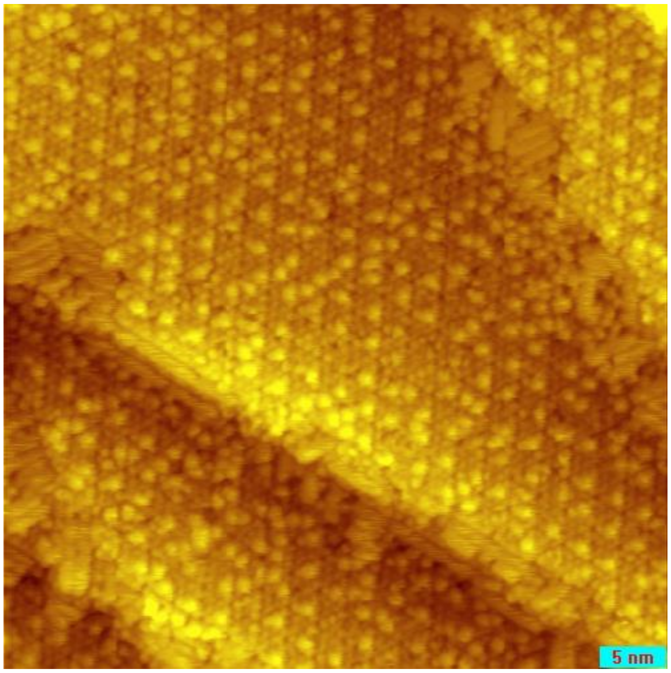


(c) 300°C annealing

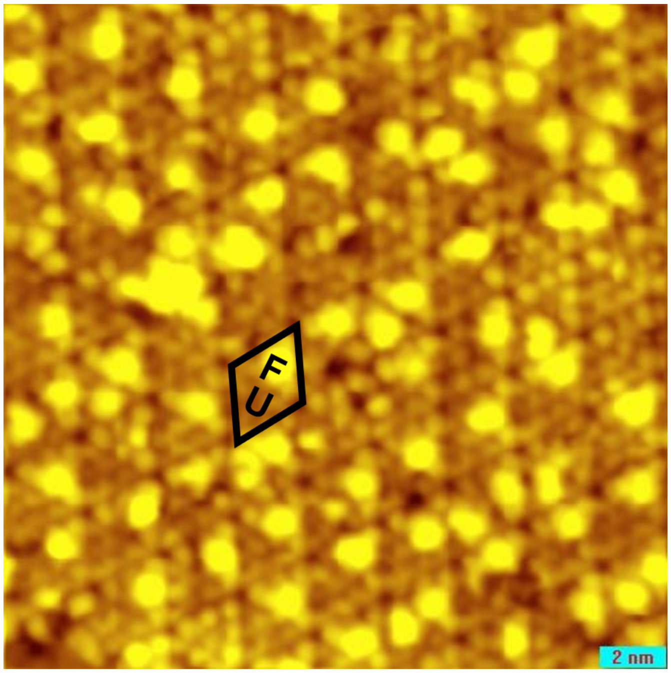


(d) 300°C annealing

FIG. S2. STM topographic images after RT deposition of Rb on the pristine Si(111)-(7 × 7) surface. (a) and (b) after Rb deposition. (c) and (d) after annealing at 300°C. Image parameters: (a), (b) −1.5 V, 0.8 nA, and (c), (d) −2.5 V, 40 pA. Image size: (a), (c) 50 nm × 50 nm, and (b), (d) 20 nm × 20 nm. The (7 × 7) unit cell is indicated in the STM images. F: faulted, U: unfaulted.

due to the annealing.

### C. (3 × 1) reconstruction

After the annealing step at 300°C, the presence of a new ordered phase on the surface, near the terraces step

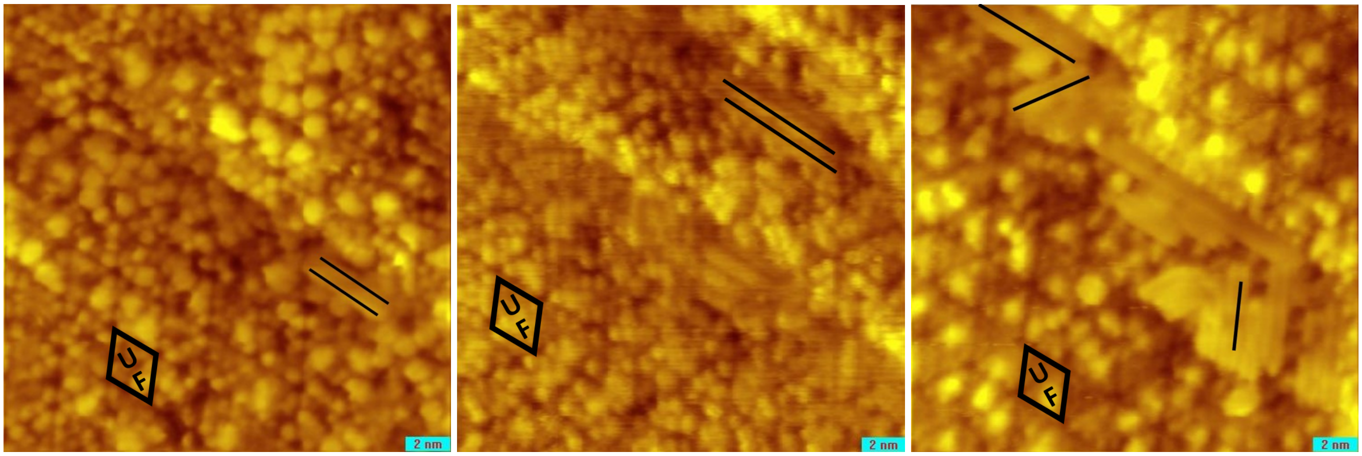


(a) (b) (c)

FIG. S3. STM topographic images (20 nm × 20 nm scan areas) measured after an annealing at 300℃ of samples obtained by room temperature Rb deposition on the pristine Si(111)-(7×7) for (a) 5 min, (b) 10 min, and (c) 15 min. Image parameters: −2.5 V, 40 pA. Double bonded chains as well as the (7 × 7) unit cell are indicated. F: faulted, U: unfaulted.

edges, was readily revealed by STM. At low amount of deposited Rb (5 min), the surface presented just few isolated double bounded chains, i.e. (3×1) domains one unit cell large (see Fig. S3(a)). By increasing the amount of evaporated Rb (10 min), the (3 × 1) domains increased in size, and the number of domains increased as well (see Fig. S3(b)). High dosing times (15 min) allowed to form larger domains. These domains could be found in all three possible orientations, as highlighted in Fig. S3(c).

Even though the presence of a (3 × 1) phase became clear at high dosing time, in rather small domains, the amount of converted surface areas did not exceed a few percent of the total surface area. This explains why no diffraction patterns other than the (7×7) could be found in the LEED experiments.
